# Supplementary material for: Integrating Pretrained Language Model for Dialogue Policy Learning
Source: arXiv:2111.01398 source file (2021-11-02)
Supplement: Supplementary file 1 [file appendix.tex]

\section{Appendix}

\begin{table*}[t]
    \centering
    \begin{tabular}{l|cccccc}
    \toprule[1pt]
    \multirow{2}{*}{Model} &  \multicolumn{6}{c}{Agenda} \\\cline{2-7}
     & Turns (succ/all) & Precision & Recall & F1 & Match & Success \\
    \hline
    \textbf{Human}  & 11.34/ 11.84 & 81.9 & 93.4 & 85.3 & 92.1 & 82.7 \\
    \hline
    MLE & 12.61/19.44 & 63.1 & 72.6 & 64.5 & 50.1 & 47.0 \\
    GDPL & \textbf{11.91}/19.28 & 63.1 & 73.0 & 64.6 & 50.0 & 47.2 \\
    PPO & 13.05/18.16 & 64.4 & 78.3 & 68.2 & 64.7 & 61.2 \\
    \hline
    PPO-OFF-Human & 12.18/17.89 & 63.0 & 81.2 & 67.8 & 70.8 & 63.2 \\
    PPO-OFF-BERT & 12.74/\textbf{16.61} & 60.9 & 82.9 & 67.4 & 70.9 & 67.6 \\
    PPO-OFF-Comb & 12.72/16.66 & \textbf{67.2} & \textbf{85.7} & \textbf{72.7} & \textbf{79.6} & \textbf{71.4} \\
    \bottomrule[1pt]
    \end{tabular}
    \caption{Performance of different dialog agents on the multi-domain dialog corpus by interacting with the agenda-based user simulator. Success average turns / all average turns}
    \label{tab:exp_res}
\end{table*}

\begin{table}[t]
    \centering
    \begin{tabular}{l|ccc}
    \toprule[1pt]
    \multirow{2}{*}{Model} &  \multicolumn{3}{c}{Agenda} \\ 
    \cline{2-4} & Precision/Recall/F1 & Match & Success \\
    \hline
    \textbf{Human}  & 81.9/93.4/85.3 & 92.1 & 82.7 \\
    \hline
    MLE  & 63.1/72.6/64.5 & 50.1 & 47.0 \\
    GDPL  & 63.1/73.0/64.6 & 50.0 & 47.2 \\
    PPO & 64.4/78.3/68.2 & 64.7 & 61.2 \\
    \hline
    PPO-OFF-Human  & 63.0/81.2/67.8 & 70.8 & 63.2 \\
    PPO-OFF-BERT & 60.9/82.9/67.4 & 70.9 & 67.6 \\
    PPO-OFF-Comb & \textbf{67.2}/\textbf{85.7}/\textbf{72.7} & \textbf{79.6} & \textbf{71.4} \\
    \bottomrule[1pt]
    \end{tabular}
    \caption{Performance of different dialog agents on the multi-domain dialog corpus by interacting with the agenda-based user simulator. Success average turns / all average turns}
    \label{tab:exp_res}
\end{table}

% 伪代码 使用一个table？
\begin{algorithm}[t]
\caption{Evaluation of Dialogue Policy Learning}
\label{alg1}
\begin{algorithmic}[1] \footnotesize
\REQUIRE ~~\\
Action pairs $(a_1 a_2)$ from expert demonstrations, $C$ \\
\STATE initialize $\pi(s, a; \theta_\pi)$ and $Q(s,a;\theta_Q)$ by supervised learning
\STATE train a classifier $f(a_u, a_s)$ according to Eq. 4.  
\STATE initialize trajectory memory buffer $D = []$
\FOR{each iteration}
\STATE user acts $a_u$
\STATE initialize state $s$
\WHILE{$s$ is not terminal state}
\STATE system decides next action $a_s$ according to $\pi(a_t | s; \theta)$
\STATE // integrate classifier to evaluate the action decision
\STATE given user action $a_u$ and system action $a_s$ as input for the trained classifier $f$ to get score $r_{classifier}$ (Eq. 6)
\STATE receive the reward $r_{human}$ and switch to a new state $s'$
\STATE // integrate classifier to shape the reward
\IF{only human reward}
\STATE store $(s, a_s, r_{human}, s')$ to the memory buffer
\ELSIF{only classifier reward} 
\STATE $r_{classifier} = -1 + 2 * r_{classifier}$
\STATE store $(s, a_s, r_{classifier}, s')$ to the memory buffer
\ELSIF{both reward} 
\STATE $r_{classifier} = -1 + 2 * r_{classifier}$
\STATE store $(s, a_s, r_{classifier} + r_{human}, s')$ to the memory buffer $D$
\ENDIF
\STATE $s = s'$
\ENDWHILE
\STATE sample minibatches of $(s, a, r, s')$ from $D$
\STATE update $\theta_Q$ according to Eq. 7
\STATE each every $C$ iterations set $\theta_Q' = \theta_Q$
\ENDFOR
\end{algorithmic}
\label{algo:eva}
\end{algorithm}
